# Supplementary material for: Unsupervised Intuitive Physics from Past Experiences
Source: arXiv:1905.10793 source file (2019-05-26)
Supplement: Supplementary file 1 [file appendix.tex]

\setcounter{section}{0}

\setcounter{table}{0}

\setcounter{figure}{0}

\section{Data generation}
In~\cref{fig:dataset} we provide more details on the scene aspect. For solid background color, the objects and background colours are sampled to be different. Every rectangular object have height and width randomly sample in between 10 and 17 pixels. Custom object are loaded from template images and randomly scaled from 1 to 2. 
\begin{figure}[h]
    \centering
    \includegraphics[width=0.3\linewidth,height=9.3em]{images/supp/colors.jpg}
    \includegraphics[width=0.3\linewidth]{images/supp/texture.jpg}
    \includegraphics[width=0.24\linewidth]{images/supp/bump_all.png}
    \caption{\textbf{Additional material used for data generation}. From left to right: color palette for solid object/background color (R2,R4,C), texture used to increase background complexity in (C+T), set of custom objects for (C) data generation.}
    \label{fig:dataset}
\end{figure}{}

\section{Implementation details}
\subsection{Network architecture}
In \cref{f:net} we show the details of all the networks of our pipeline. The regression network mentionned in sec.5 is a simple 3 layers fully convolutional network with [3x3] kernel convolution and intermediate channel of size 64.
\begin{figure}
\centering\includegraphics[width=\textwidth]{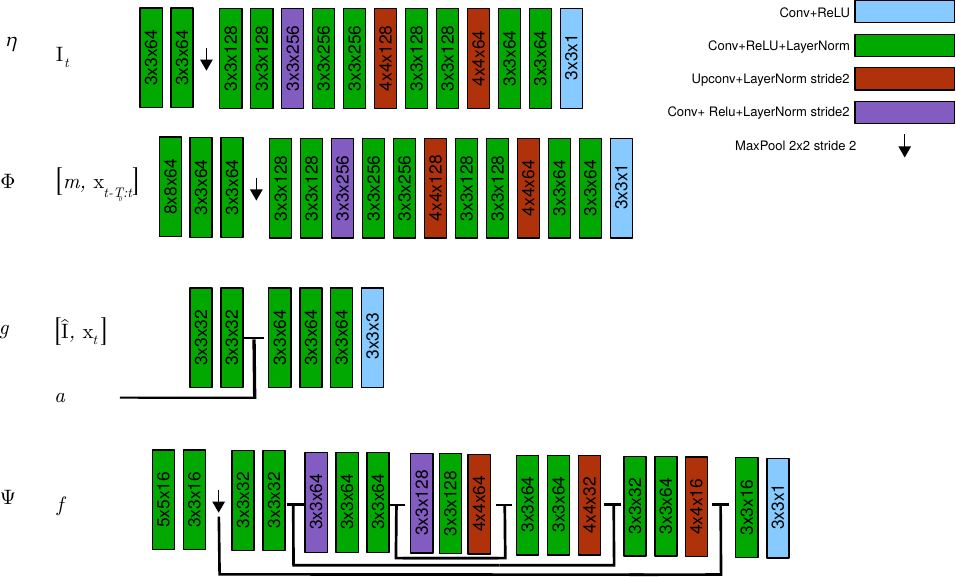}
\caption{\textbf{Networks architecture detail}. All the networks generally uses layer normalization $\eta$ and $\Phi$ are simple auto-encoder type architecture while $\Psi$ shares similarity with U-Net.}\label{f:net}  
\end{figure}

\subsection{Training details}
In the overall loss $l$ is:
$$
\ell(t) = 
\lambda_{\mathbf{I}}\|
\mathbf{I}_t - \hat{\mathbf{I}}_t
\|^2
+
\lambda_{\mathbf{x}}\|\mathbf{x}_t - \eta(\mathbf{I}_t(\mathcal{R}))\|^2
+
\lambda_{p}\| 
e(\mathbf{I}_t) - e(\hat{\mathbf{I}}_t)
\|^2
$$
When training without $L^2$ we used $\lambda_{\mathbf{I}}=\lambda_{\mathbf{x}}=1$. When finetuning with perceptual we weighted the perceputal loss with coefficient $\lambda_{perc}=10$ and the other losses with $\lambda_{\mathbf{I}}=\lambda_{\mathbf{x}}=0.01$. Finally, perceptual loss uses feature extracted from conv3 of VGG-16.

The Interaction Network baseline is a simple Interaction Network to which state we concatenated the background feature extracted from a pre-trained VGG-16 network. The state propagator uses the last 4 states. The network is then trained over $T_{train}=40$ time steps with Adam optimizer with learning rate $10^{-4}$ and batch size 50.  We found that 50 000 iterations were sufficient to reach convergence.

All  experiments are run using single NVIDIA-GPU Titan X.
\subsection{Evaluation details}
To detect blob create a binary image by manually thresholding the intermediate heatmap $\mathbf{x}_t$ and using a simple Hough circle detector. Every threshold coefficient is hand picked for every model but kept constant across scenarios and different data.
\section{Additional results}
\begin{table*}[t]
\centering
\scriptsize
\newcommand{\xpm}[1]{{\tiny$\pm$#1}}
\setlength{\tabcolsep}{0.5em}
\caption{\textbf{Importance of experience.} For the \textbf{supervised} model, we report the trajectory prediction error at $T=40$ (rows 1-3) and the obstacle map prediction error (rows 4-6) for different obstacle types.
The number of runs $N$ in the experiences is varied from 0 to 50.
%Values have been normalized by the board size diagonal.
Position errors were normalized by the board size diagonal. $T_\text{train} = 20$.
}\label{t:num_runs_pos}
\begin{tabular}{cllcccccccc}
\toprule
No  & Err. &  Obst.    & $N            = 0$            & $1$           & $2$           & $5$           & $7$           & $10$          & $20$ & $50$\\ 
\midrule
(1) & Pos. & R2   & 1.81\xpm{1.41} & .94\xpm{.975} & .53\xpm{.81} & .15\xpm{0.41}  & .08\xpm{.21}   & .07\xpm{.16}  & .10\xpm{.24}   & .19\xpm{.38} \\
(2) & Pos. & R4 & 3.28\xpm{1.94}  & 2.22\xpm{1.67} & 1.56\xpm{1.40} & .63\xpm{.84} & .43\xpm{.68} &  .37\xpm{.60} & .44\xpm{.61} & .83\xpm{.97}\\
(3) & Pos. &  C      & 1.05\xpm{0.91} & .58\xpm{.61} & .36\xpm{.49} & .15\xpm{.29} & .13\xpm{.26} & .12\xpm{.22} &  .16\xpm{.26} & .24\xpm{.36}\\
\midrule
(4) & Obs. &  R2   & 4.1\xpm{4.0} & 3.6\xpm{3.8} & 3.1\xpm{3.4 }& 2.3\xpm{2.5}  & 2.3\xpm{2.4}  & 2.3\xpm{2.4}  & 2.3\xpm{2.7}   & 2.6\xpm{3.0} \\
(5) & Obs. & R4 & 6.1\xpm{2.2}  & 4.1\xpm{3.8} & 3.1\xpm{3.4} & 2.8\xpm{3.3} & 2.7\xpm{3.1} & 2.6\xpm{3.0} & 2.7\xpm{2.9} & 3.3\xpm{3.6}\\
(6) & Obs. & C      & 3.9\xpm{3.9}  & 3.3\xpm{3.7} & 2.8\xpm{3.1} & 2.4\xpm{2.7} & 2.4\xpm{2.8} & 2.3\xpm{2.6} & 2.4\xpm{2.6} & 2.5\xpm{2.9}\\

%(4) & Obs. &  R2   & .178\xpm{.175} & .142\xpm{.160} & .107\xpm{.126 }& .060\xpm{.072}  & .056\xpm{.064}  & .056\xpm{.063}  & .061\xpm{.082}   & .075\xpm{.100} \\
%(5) & Obs. & R4 & .409\xpm{.053}  & .190\xpm{.158} & .107\xpm{.126} & .087\xpm{.118} & .801\xpm{.103} & .078\xpm{.103} & .081\xpm{.096} & .120\xpm{.140}\\
%(6) & Obs. & C      & .166\xpm{.171}  & .122\xpm{.152} & .084\xpm{.108} & .061\xpm{.078} & .640\xpm{.088} & .061\xpm{.072} & .061\xpm{.074} & .072\xpm{.096}\\
\bottomrule
\end{tabular}
\end{table*}

\if0
\begin{table*}[t]
\centering
\scriptsize
\newcommand{\xpm}[1]{{\tiny$\pm$#1}}
\setlength{\tabcolsep}{0.5em}
\caption{\textbf{Importance of experience.} For the \textbf{supervised} model, we report the trajectory prediction error at $T=40$ (rows 1-3) and the obstacle map prediction error (rows 4-6) for different obstacle types.
The number of runs $N$ in the experiences is varied from 0 to 50.
Values have been normalized by the board size diagonal.
}\label{t:num_runs_pos}
\begin{tabular}{cllcccccccc}
\toprule
No  & Err. &  Obst.    & $N            = 0$            & $1$           & $2$           & $5$           & $7$           & $10$          & $20$ & $50$\\ 
\midrule
(1) & Pos. & R2   & 1.81\xpm{1.41} & .94\xpm{.975} & .53\xpm{.81} & .15\xpm{0.41}  & .08\xpm{.21}   & .07\xpm{.16}  & .10\xpm{.24}   & .19\xpm{.38} \\
(2) & Pos. & R4 & 3.28\xpm{1.94}  & 2.22\xpm{1.67} & 1.56\xpm{1.40} & .63\xpm{.84} & .43\xpm{.68} &  .37\xpm{.60} & .44\xpm{.61} & .83\xpm{.97}\\
(3) & Pos. &  C      & 1.05\xpm{0.91} & .58\xpm{.61} & .36\xpm{.49} & .15\xpm{.29} & .13\xpm{.26} & .12\xpm{.22} &  .16\xpm{.26} & .24\xpm{.36}\\
\midrule
(4) & Obs. &  R2   & 16.9\xpm{15.9} & 12.9\xpm{14.5} & 9.7\xpm{11.4 }& 5.4\xpm{6.5}  & 5.1\xpm{5.8}  & 5.1\xpm{5.8}  & 5.5\xpm{7.4}   & 6.8\xpm{9.1} \\
(5) & Obs. & R4 & 37.0\xpm{4.8}  & 17.2\xpm{14.3} & 9.7\xpm{11.4} & 7.9\xpm{10.7} & 7.1\xpm{9.4} & 7.0\xpm{9.3} & 7.4\xpm{8.7} & 10.9\xpm{12.7}\\
(6) & Obs. & C      & 15.0\xpm{15.5}  & 11.1\xpm{13.8} & 7.6\xpm{9.8} & 5.6\xpm{7.1} & 5.8\xpm{8.0} & 5.5\xpm{6.6} & 5.6\xpm{6.7} & 6.5\xpm{8.7}\\

%(4) & Obs. &  R2   & .178\xpm{.175} & .142\xpm{.160} & .107\xpm{.126 }& .060\xpm{.072}  & .056\xpm{.064}  & .056\xpm{.063}  & .061\xpm{.082}   & .075\xpm{.100} \\
%(5) & Obs. & R4 & .409\xpm{.053}  & .190\xpm{.158} & .107\xpm{.126} & .087\xpm{.118} & .801\xpm{.103} & .078\xpm{.103} & .081\xpm{.096} & .120\xpm{.140}\\
%(6) & Obs. & C      & .166\xpm{.171}  & .122\xpm{.152} & .084\xpm{.108} & .061\xpm{.078} & .640\xpm{.088} & .061\xpm{.072} & .061\xpm{.074} & .072\xpm{.096}\\
\bottomrule
\end{tabular}
\end{table*}
\fi
%\begin{table*}[t]
%  \centering
%  \caption{\textbf{Tempral invariance on Normal-3 balls unsupervised}, Number of balls over time}\label{t:normal-1ball-uns}
%  %\vspace{-1em}
%  \scriptsize
%  \setlength{\tabcolsep}{0.4em}
%
%  \sisetup{detect-weight=true,detect-inline-weight=math,  table-column-width=4.2em}
%  \newcommand{\boldentryy}[2]{%
%  \multicolumn{1}{S[table-format=0.3,
%                      mode=text, text-rm=\fontseries{b}\selectfont
%                     ]#2}{#1}}
%  \newcolumntype{F}{S[table-format=0.3,table-column-width=4.2em]}
%  \begin{tabular}{ccccc}
%  \toprule
%      & \multicolumn{4}{c}{Normal-3 ball-\Ttrain=20}\\
%      Method &
%     \multicolumn{1}{c}{$T=$6} & \multicolumn{1}{c}{$T=$\Ttrain} &    \multicolumn{1}{c}{$3\times$\Ttrain} & 
%      \multicolumn{1}{c}{$5\times$\Ttrain}\\ 
%      64x64 + 1 ball trained + Perc. loss & 3.1 $\pm$0.5 & 2.8$\pm$0.9 & 1.7$\pm$0.8 & 1.5$\pm$0.8\\
%  %    \midrule
%  \end{tabular}
%  \end{table*}

\begin{table*}[t]
\centering
\footnotesize
\newcommand{\xpm}[1]{{\tiny$\pm$#1}}
\caption{\textbf{Predicting multiple moving object.} Obstacle type is R2, all network were trained on the fully unsupervised with perceptual loss. Num. is the maxmium number of balls per run during training. For instance Num=3 means that every runs sampled contained one to three balls.
The test board is size $64\times 64$
We test the average prediction error at $T_{\text{test}}=20,60,100$ well above the duration $T_\text{train}=20$ observed during training.
}
\label{t:normal-mul-uns}
\setlength{\tabcolsep}{0.21em}
\begin{tabular}{c*2c*2c*2c}
\toprule
& \multicolumn{2}{c}{$T_\text{test} = T_{\text{train}} = 20$} & \multicolumn{2}{c}{$T_\text{test} = 3\times$\Ttrain} &  \multicolumn{2}{c}{$T_\text{test}=5\times$\Ttrain}\\ 
\cmidrule(lr){2-3} \cmidrule(lr){4-5} \cmidrule(lr){6-7}\\
Num.  & \# obj.     & Vid.~$L_2$    & \# obj.      & Vid.~$L_2$      &  \# obj.      & Vid.~$L_2$      \\
\midrule
\multicolumn{7}{c}{3 Balls}\\
\midrule
1  & 2.6\xpm{0.8} & 6.5\xpm{5.2}  &  1.7\xpm{0.9}  & 8.5\xpm{5.9}    & 1.6\xpm{0.8}  & 8.5\xpm{6.0}  \\
3 &  3.1\xpm{0.6} & 4.6\xpm{4.8} & 2.9\xpm{0.8}  & 10.4\xpm{7.6}   & 2.9\xpm{0.9}  & 11.0\xpm{8.0} \\
\midrule
\multicolumn{7}{c}{5 Balls}\\\midrule

1  & 3.3\xpm{1.0} & 8.9\xpm{6.6}   & 2.0\xpm{1.0}  & 10.2\xpm{7.4}   &  3.1\xpm{0.6}  & 1.8\xpm{.775}  \\
3 &  5.5\xpm{0.7} & 6.6\xpm{6.2} & 5.1\xpm{1.1}  & 13.0\xpm{9.5}   &  5.1\xpm{1.0}  & 13.5\xpm{10.0} \\
%\multicolumn{7}{c}{3 Balls}\\
%\midrule
%1  & 2.6\xpm{0.8} & .46\xpm{.30}  & 1.7\xpm{0.9}  & .8\xpm{.39}   & 1.6\xpm{0.8}  & .79\xpm{.40} \\
%3 &  3.1\xpm{0.6} & .23\xpm{.26}& 2.9\xpm{0.8}  & 1.20\xpm{.63}  & 2.9\xpm{0.9}  & 1.35\xpm{.71} \\
%\midrule
%\multicolumn{7}{c}{5 Balls}\\
%\midrule
%
%1  & 3.3\xpm{1.0} & .88\xpm{.48}   & 2.0\xpm{1.0}  & 1.15\xpm{.61} & 3.1\xpm{0.6}  & 1.17\xpm{.65} \\
%3 &  5.5\xpm{0.7} & .49\xpm{.42} & 5.1\xpm{1.1}  & 1.85\xpm{.99}   &  5.1\xpm{1.0}  & 2.03\xpm{1.11} \\
\bottomrule
\end{tabular}
\end{table*}

\if0 %BEFORE RENORM
\begin{table*}[t]
\centering
\footnotesize
\newcommand{\xpm}[1]{{\tiny$\pm$#1}}
\caption{\textbf{Predicting multiple moving object.} Obstacle type is R2, all network were trained on the fully unsupervised with perceptual loss. Num. is the maxmium number of balls per run during training. For instance Num=3 means that every runs sampled contained one to three balls.
The test board is size $64\times 64$
We test the average prediction error at $T_{\text{test}}=20,60,100$ well above the duration $T_\text{train}=20$ observed during training.
Video prediction error has been normalized by the board size diagonal.
}
\label{t:normal-mul-uns}
\setlength{\tabcolsep}{0.21em}
\begin{tabular}{c*2c*2c*2c}
\toprule
& \multicolumn{2}{c}{$T_\text{test} = T_{\text{train}} = 20$} & \multicolumn{2}{c}{$T_\text{test} = 3\times$\Ttrain} &  \multicolumn{2}{c}{$T_\text{test}=5\times$\Ttrain}\\ 
\cmidrule(lr){2-3} \cmidrule(lr){4-5} \cmidrule(lr){6-7}\\
Num.  & \# obj.     & Vid.~$L^2$    & \# obj.      & Vid.~$L^2$      &  \# obj.      & Vid.~$L^2$      \\
\midrule
\multicolumn{7}{c}{3 Balls}\\
1  & 2.6\xpm{0.8} & 42.11\xpm{27.2}  &  1.7\xpm{0.9}  & 72.4\xpm{35.4}    & 1.6\xpm{0.8}  & 72.0\xpm{36.6}  \\
3 &  3.1\xpm{0.6} & 21.2\xpm{23.3} & 2.9\xpm{0.8}  & 108.4\xpm{57.4}   & 2.9\xpm{0.9}  & 122.0\xpm{63.8} \\
\midrule
\multicolumn{7}{c}{5 Balls}\\\midrule

1  & 3.3\xpm{1.0} & 79.5\xpm{43.8}   & 2.0\xpm{1.0}  & 104.7\xpm{55.3}   &  3.1\xpm{0.6}  & 3.1\xpm{0.6}  \\
3 &  5.5\xpm{0.7} & 44.2\xpm{38.2} & 5.1\xpm{1.1}  & 168.2\xpm{90.0}   &  5.1\xpm{1.0}  & 183.6\xpm{100.8} \\
%\multicolumn{7}{c}{3 Balls}\\
%\midrule
%1  & 2.6\xpm{0.8} & .46\xpm{.30}  & 1.7\xpm{0.9}  & .8\xpm{.39}   & 1.6\xpm{0.8}  & .79\xpm{.40} \\
%3 &  3.1\xpm{0.6} & .23\xpm{.26}& 2.9\xpm{0.8}  & 1.20\xpm{.63}  & 2.9\xpm{0.9}  & 1.35\xpm{.71} \\
%\midrule
%\multicolumn{7}{c}{5 Balls}\\
%\midrule
%
%1  & 3.3\xpm{1.0} & .88\xpm{.48}   & 2.0\xpm{1.0}  & 1.15\xpm{.61} & 3.1\xpm{0.6}  & 1.17\xpm{.65} \\
%3 &  5.5\xpm{0.7} & .49\xpm{.42} & 5.1\xpm{1.1}  & 1.85\xpm{.99}   &  5.1\xpm{1.0}  & 2.03\xpm{1.11} \\
\bottomrule
\end{tabular}
\end{table*}
\fi
